# Supplementary material for: Dynamical formation and interaction-induced stabilization of dark condensates of dipolar excitons
Source: arXiv:1803.03918 source file (2018-05-07)
Supplement: Supplementary file 1 [file si-dynamical-formation.pdf]

# Dynamical formation and interaction-induced stabilization of dark condensates of dipolar excitons

## Supplementary Material

Yotam Mazuz-Harpaz,[1] Maxim Khodas,[1] and Ronen Rapaport[1,2,*]

[1] *Racah Institute of Physics, Hebrew University of Jerusalem, Jerusalem 91904, Israel*

[2] *Applied Physics Department, Hebrew University of Jerusalem, Jerusalem 91904, Israel*

### S1. WAVE VECTOR DEPENDENCE OF $\xi_d$

Eq. 5 of the main text defines $\Phi_d$, the wavefunction of the relative position of two colliding IXs. While generally dependent on the collision wave number $k$, this dependence is in fact negligible in the case of a an extended condensate. We note that $K_0(z) \simeq -\ln(z/2)$ for $|z| \ll 1$. $|z| \ll 1$ corresponds to the condition $2\pi/k \gg 4d^2/b$ in Eq. 5. Thus in this range, the dependence of $\Phi_d$ on $k$ is logarithmically small. This means that for an IX condensate with a typical size $L \sim 10\mu m$, $2\pi/k \sim L \gg 4d^2/b$ , and $\Phi_d$ is practically independent of $k$. This is demonstrated in Fig. S1, showing the exchange integral $\xi_d$ vs. $2\pi/k$ for several dipole lengths.

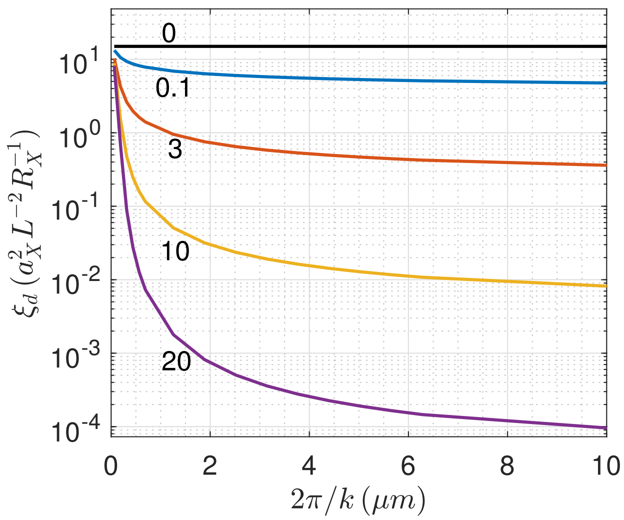


FIG. S1. The exchange integral $\xi_d$ vs. the inverse of the scattering wave vector $2\pi/k$ for several dipole moments, specified in nm. Calculated using the typical values for IX systems, $a_X = 10$nm and $b = 3$nm, and $\Phi_d$ of Eq. 5 of the main text.

### S2. RELAXATION DYNAMICS OF A CONDENSATE

The decay dynamics of an IX population is described by Eq. 10 of the main text, with $G = 0$:

$$\frac{d}{dt}\bar{N} = -\gamma N - \gamma_{th} N_{th}. \tag{S1}$$

* ronenr@phys.huji.ac.il

When the condensate is in a mixed state (see main text), $\bar{N} > \bar{N}_{c1} + N_{c2}$, then substituting $\gamma = (\gamma_{nr} N_D + \gamma_r N_B)/N$ and Eqs. 1 and 2 of the main text into Eq. S1 we get:

$$\begin{aligned} \frac{d}{dt}\bar{N} &= \frac{\gamma_{nr}}{2}\left(\bar{N} - N_{th} + N_{c2}\right) + \frac{\gamma_r}{2}\left(\bar{N} - N_{th} - N_{c2}\right) - \gamma_{th} N_{th} \\ &= -\gamma_{th}\bar{N} + \frac{1}{2}\gamma_r N_{c2}. \end{aligned} \tag{S2}$$

When $\bar{N}_{c1} + N_{c2} > \bar{N} > \bar{N}_{c1}$ the condensate is dark, in which case:

$$\frac{d}{dt}\bar{N} = -\gamma_{nr}\bar{N} - \frac{1}{2}\gamma_r N_{th}. \tag{S3}$$

Finally, when $\bar{N} < \bar{N}_{c1}$ the condensate is fully depleted leaving only a thermal cloud that decays according to:

$$\frac{d}{dt}\bar{N} = -\gamma_{th}\bar{N}. \tag{S4}$$

Solving Eqs. S2, S3 and S4, for the case $\bar{N}(t=0) = \bar{N}_0 > \bar{N}_{c1} + N_{c2}$ the population decay is given by:

$$\bar{N}(t) = \begin{cases} \left(\bar{N}_0 - \frac{\gamma_r}{2\gamma_{th}} N_{c2}\right) e^{-\gamma_{th} t} + \frac{\gamma_r}{2\gamma_{th}} N_{c2} & t_1 > t \\ \left(\bar{N}_{c1} + N_{c2}\right) e^{-\gamma_{nr}(t-t_1)} - \frac{\gamma_r}{2\gamma_{nr}} \bar{N}_{c1} & t_2 > t > t_1 \\ \bar{N}_{c1} e^{-\gamma_{th}(t-t_2)} & t > t_2 \end{cases} \tag{S5}$$

where $t_1$ and $t_2$ are the times corresponding to the transitions from a mixed condensate to a dark condensate and from a dark condensate to a pure thermal distribution, respectively:

$$t_1 = \frac{1}{\gamma_{th}} \log\left[\frac{\gamma_{th}\bar{N}_0 - \frac{1}{2}\gamma_r N_{c2}}{\gamma_{th}\bar{N}_{c1} + \gamma_{nr} N_{c2}}\right] \tag{S6}$$

$$t_2 = t_1 + \frac{1}{\gamma_{nr}} \log\left[\frac{\gamma_{nr} N_{c2}}{\gamma_{th}\bar{N}_{c1}} + 1\right]. \tag{S7}$$

This unique dynamics of IX fluids can be observed directly by time-resolved PL measurements. The expected PL intensity, $I$, is proportional to the number of the bright particles

$$I \propto \bar{N}_B = N_B + N_{th}/2. \tag{S8}$$

$\bar{N}_B$ can be found from Eq. S5 and Eq. 1 of the main text, yielding:

$$2\bar{N}_B = \begin{cases} \left(\bar{N}_0 - \frac{\gamma_r}{2\gamma_{th}} N_{c2}\right) e^{-\gamma_{th} t} - \frac{\gamma_{nr}}{\gamma_{th}} N_{c2} & t_1 > t \\ \bar{N}_{c1} & t_2 > t > t_1 \\ \bar{N}_{c1} e^{-\gamma_{th}(t-t_2)} & t > t_2. \end{cases} \tag{S9}$$

Both Eqs. S5 and S9 are illustrated by Figure 3(c) of the main text.
